# Supplementary material for: State-resolved infrared spectrum of the protonated water dimer: Revisiting the characteristic proton transfer doublet peak
Source: arXiv:2206.12029 ancillary file (2022-09-05)
Supplement: Supplementary file 1 [file ESI.pdf]

# Supporting information for: "State-resolved infrared spectrum of the protonated water dimer: Revisiting the characteristic proton transfer doublet peak"

Henrik R. Larsson,[1,2] Markus Schröder,[3] Richard Beckmann,[4] Fabien Brieuc,[4,a)] Christoph Schran,[4,b)] Dominik Marx,[4] and Oriol Vendrell[3]

[1)]Department of Chemistry and Biochemistry, University of California, Merced, CA 95343, USA

[2)]Division of Chemistry and Chemical Engineering, California Institute of Technology, Pasadena, CA 91125, USA

[3)]Theoretische Chemie, Physikalisch-Chemisches Institut, Universität Heidelberg, Im Neuenheimer Feld 229, D - 69120 Heidelberg, Germany

[4)]Lehrstuhl für Theoretische Chemie, Ruhr-Universität Bochum, 44780 Bochum, Germany

## S1. SETUP

We use the same basis and polyspherical coordinates as Vendrell et al.[1–3]. The names and basis size of the used coordinates are shown in Table S1.

TABLE S1. Coordinates of the Zundel cation and their basis size.

| Symbol | basis size | meaning |
|---|---|---|
| $R$ | 20 | water-water stretch |
| $z$ | 19 | proton transfer |
| $x$ | 7 | |
| $y$ | 7 | |
| $\alpha$ | 11 | water rotation |
| $\gamma_a$ | 19 | water wagging |
| $\gamma_b$ | 19 | |
| $\beta_a$ | 9 | water rocking |
| $\beta_b$ | 9 | |
| $r_{1a}$ | 9 | water *a* |
| $r_{1b}$ | 9 | |
| $\theta_a$ | 9 | |
| $r_{2a}$ | 9 | water *b* |
| $r_{2b}$ | 9 | |
| $\theta_b$ | 9 | |

### A. Tensor Tree

Both the tensor tree network state TTNS[4] and the PES representations (see Section S4) uses the same mode combination, that is, several coordinates are combined to "logical" coordinates to decrease the dimensionality of the problem from 15 to 6. Mode combination is used because the previous multiconfiguration time-dependent Hartree (MCTDH) simulations[1–3] benefited from it. This is not necessarily the case for multilayer (ML) MCTDH and TTNSs but cumbersome attempts to refit the PESs without mode combination have not been done.

Due to the limit overall dimensionality of the system, we did not use a sophisticated tree with many layers but rather use a so-called Tucker matrix product state (MPS), as displayed in Fig. S1. A Tucker MPS is a MPS with additional transformation matrices added to the legs of the MPS, shown in green in Fig. S1. These transformation matrices are added to reduce the overall size of each tensor, which is required because the basis size of the logical coordinates is very large (up to 729), compared to the used bond dimension $D$ (size here between 50 and 150). Transformation matrices have not been added to the ends of the MPS because there the tensors are two dimensional and overall have small size (see Ref. [5] for a detailed discussion). We optimized the order of the six logical coordinates using the procedure from Ref. [4].

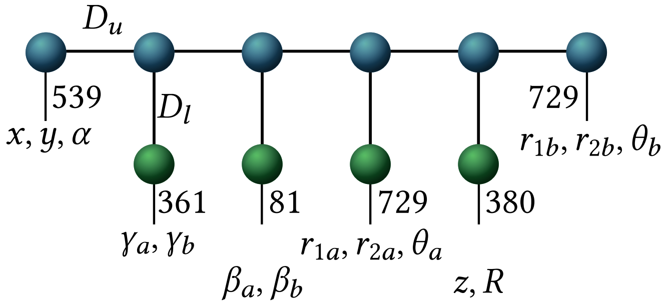


FIG. S1. Topology of the tensor tree used in the simulations. Displayed are the coordinates and the combined basis size. $D_u$ ($D_l$) is the bond dimension of the upper (lower) tree.

### B. Eigenstate optimization

We use a density matrix renormalization group-like procedure to optimize the TTNS for each eigenstate. See Ref. [4] for a detailed discussion of the used procedure. For each eigenstate the bond dimensions $D$ are adjusted based on a singular value threshold $\epsilon$, which we set to $10^{-6}$. In addition, we fixed the maximal used bond dimension $D_{\max}$ to be either 50, 70, 100, or 150. For Fig. 1 in the main text, on the BBSM surface, we used $D_{\max} = 100$ for the lowest 383 states up to 1510 cm$^{-1}$, followed by $D_{\max=70}$ for the lowest 540 states up to 1665 cm$^{-1}$. On the HBB surface, we used $D_{\max} = 150$ for the lowest 150

[a)]Current Address:Laboratoire Matière en Conditions Extrêmes, Université Paris-Saclay, CEA, DAM, DIF, 91297 Arpajon, France
[b)]Current Address:Yusuf Hamied Department of Chemistry, University of Cambridge, Lensfield Road, Cambridge, CB2 1EW, UK

states up to 1107 cm$^{-1}$, followed by $D_{max=100}$ for the lowest 249 states up to 1305 cm$^{-1}$ and by $D_{max=50}$ for the lowest 892 states up to 1920 cm$^{-1}$.

To test the convergence, we compared the energies from the optimizations with larger bond dimensionsions to those with smaller bond dimensions. A comparison of the energy terms up to ∼1030 cm$^{-1}$ computed with a max. bond dimension of either 100 or 150 leads to an error of less than 1.5 cm$^{-1}$, much less than the errors of the PES representation (see Section S4). A comparison of the energy terms up to ∼ 1300 cm$^{-1}$ computed with a max. bond dimension of either 70 or 100 leads to an error of less than 8.0 cm$^{-1}$ (5 cm$^{-1}$) on the HBB (BBSM) surface.

### C. Time evolution

We generated the infrared spectrum obtained by time evolution by Fourier transforming the convoluted autocorrelation function of the dipole-operated ground state, as shown in Ref. [1]. As damping function we chose $g(t) = \cos^2(\pi t/2T)$. The final propagation times $T$ were 2742 fs for the BBSM PES and 2362 fs for the HBB PES.

The TTNSs were propagated using the time-depended DMRG-based algorithm described in Refs. [6,7]. We generated the initial wavefunction $|\Psi(t=0)\rangle = \hat{\mu}_i|\Psi_0\rangle$ by fitting the action of one of the three dipole operators $\hat{\mu}_x, \hat{\mu}_y, \hat{\mu}_z$ to the ground state $|\Psi_0\rangle$ using a DMRG-like procedure.[8] Unlike the eigenstate optimizations, to simplify the simulation, we kept bond dimensions for the MPS ($D_u$) and for the transformation matrices ($D_l$) fixed at $D_u = 50$ and $D_l = 80$, respectively.

## S2. WAVEFUNCTIONS CUT

Plotting the two-dimensional wavefunction cuts requires deciding which positions of the other coordinates need to be fixed. As positions we chose the maxima of the diagonal of the one-dimensional reduced density matrices ($\Psi^2$ integrated over all but one coordinate). In the cases where there were several maxima, we analysed all possible wavefunction cuts and chose the most representative one, typically that of the global maximum of the reduced density matrix diagonal. The particular positions are listed in Table S2.

To reveal the excitations along the water-water stretch motion ($R$), Fig. S2 shows additional cuts of the three states analysed in the main text.

TABLE S2. Positions of the cuts of the wavefunctions displayed in this work. For all wavefunctions, the following positions are the same: $x, y = 0$, $\alpha = 1.57$, $r_{1a} = 1.15$, $r_{2a} = 3$, $r_{1b} = 1.15$, $r_{2b} = 3$, $\theta_a = \theta_b = 0$, and $\beta_a = \beta_b = 0$. The angles are shown in radian. Otherwise we use atomic units.

| figure | state | cuts |
|---|---|---|
| 2 | $\Psi_a^{BBSM}$ | $R = 4.78, ,\gamma_b = 0$ |
| | $\Psi_b^{BBSM}$ | $R = 4.67, \gamma_b = 0$ |
| | $\Psi_c^{BBSM}$ | $R = 4.56, \gamma_b = 0$ |
| | $\Psi_a^{HBB}$ | $R = 4.78, \gamma_b = 0$ |
| | $\Psi_b^{HBB}$ | $R = 4.56, \gamma_b = 0$ |
| | $\Psi_c^{HBB}$ | $R = 4.67, \gamma_b = 0$ |
| 3 | $\Psi_b^{BBSM}$ | $z = 0.20, R = 4.67$ |
| | $\Psi_c^{BBSM}$ | $z = 0, R = 4.56$ |
| | $\Psi_b^{HBB}$ | $z = -0.10, R = 4.56$ |
| | $\Psi_c^{HBB}$ | $z = 0.15, R = 4.67$ |
| S2 | $\Psi_a^{BBSM}$ | $z = 0.15, \gamma_b = 0$ |
| | $\Psi_b^{BBSM}$ | $z = -0.20, \gamma_b = 0$ |
| | $\Psi_c^{BBSM}$ | $z = 0, \gamma_b = 0$ |
| | $\Psi_a^{HBB}$ | $z = 0, \gamma_b = 0$ |
| | $\Psi_b^{HBB}$ | $z = 0.10, \gamma_b = 0$ |
| | $\Psi_c^{HBB}$ | $z = -0.15, \gamma_b = 0$ |

TABLE S3. Overlap of zero-order states with the three wavefunctions $\Psi_i$ around the doublet.

| name & PES | $\tilde{E}$/cm$^{-1}$ | $\langle 1R, 02-20|\Psi\rangle^2$ | $\langle 1z|\Psi\rangle^2$ | $\langle 04-40|\Psi\rangle^2$ |
|---|---|---|---|---|
| $\Psi_a$ HBB | 897 | 0.34 | 0.09 | 0.00 |
| $\Psi_a$ BBSM | 920 | 0.46 | 0.19 | 0.00 |
| $\Psi_b$ HBB | 1043 | 0.04 | 0.20 | 0.30 |
| $\Psi_b$ BBSM | 1041 | 0.20 | 0.36 | 0.00 |
| $\Psi_c$ HBB | 1060 | 0.11 | 0.21 | 0.13 |
| $\Psi_c$ BBSM | 1095 | 0.02 | 0.00 | 0.44 |

## S3. OVERLAP WITH TESTSTATES

Following the procedure introduced in Ref. [9] we confirm our analysis of the decomposition of the eigenstates by computing the overlap of the wavefunctions with zero-order states. While there is some arbitrariness in defining these zero-order states, they nevertheless provide a semi-quantitative confirmation of the assignment. The teststates have been prepared similar to Ref. [1]. $|1z\rangle$ and $|1R\rangle$ ($|04-40\rangle$) have been generated from the 15-dimensional Hamiltonian with all but the $z$ and $R$ ($\gamma_a$ and $\gamma_b$ coordinates fixed at the maxima of the ground-state). $|02-20; 1R\rangle$ was generated by multiplying the cut of $|1R\rangle$ in $R$ onto the $|02-20\rangle$ state of the full Hamiltonian. For all states up to a transition of 1310 cm$^{-1}$, the zero-order states only had significant overlap with the ones mentioned in the main text.

Overlaps of the zero-order states with the wavefunctions considered here are shown in Table S3. The table confirms the previous, wavefunction-based analysis. While Fig. S2 displays a small contribution from $|1z\rangle$ in $\Psi_c^{HBB}$, there is no overlap between the $|1z\rangle$ zero-order state and $\Psi_c^{HBB}$. Although this could be attributed to the quality and arbitrariness of the zero-order state, a closer inspection of $\Psi_c^{HBB}$ does not reveal a significant excitations along the $1z$ modes, except for the small contribution displayed in Fig. S2. Interestingly, compared to $\Psi_a^{HBB}$ and $\Psi_b^{HBB}$, the $|1z\rangle$ state is more dominant in $\Psi_a^{BBSM}$ and $\Psi_b^{BBSM}$. This can be attributed to the missing contributions from $|04-40\rangle$ for these states.

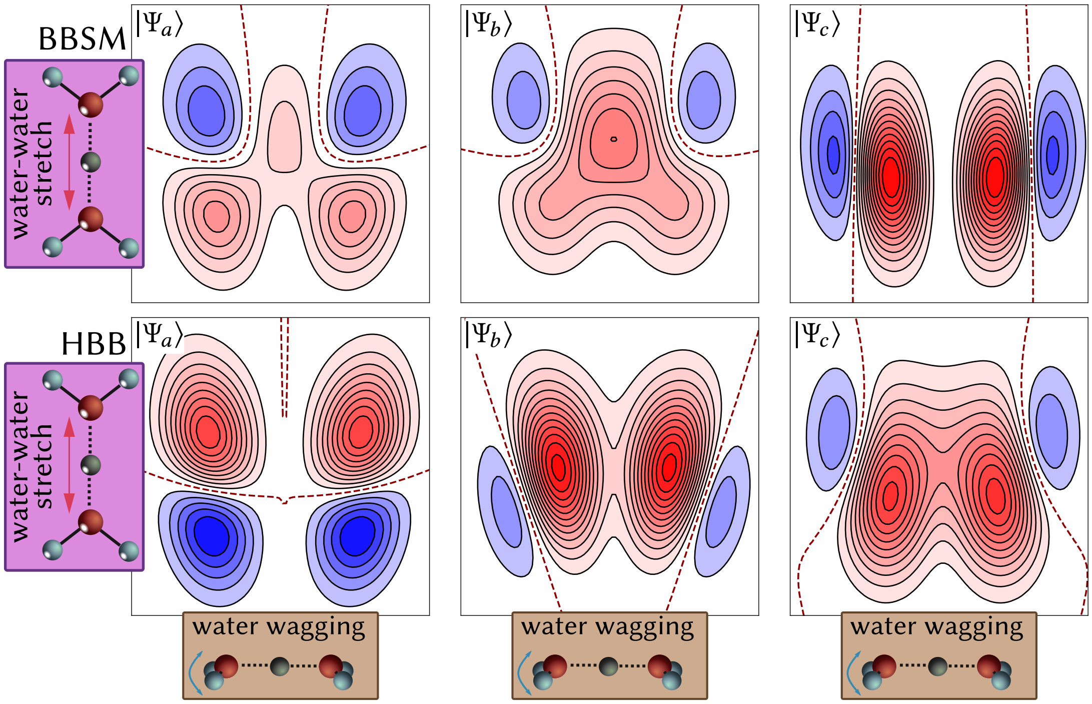


FIG. S2. Representative cuts of the wavefunctions corresponding to either the doublet and a satellite peak (BBSM, upper panels), or the triplet (HBB PES, lower panels) in the IR spectrum. Panel ($i$) corresponds to wavefunction $\Psi_i$, see text for details. The abscissa shows the wagging (pyramidalization) motion of one of the water molecules. The ordinate shows the water-water stretch motion. The red lines denote the zero contours.

## S4. FITTING OF THE POTENTIAL ENERGY SURFACE AND DIPOLE MOMENTS IN SUM-OF-PRODUCTS FORM

The multi-dimensional potential and dipole moment surfaces are expressed in the form of a canonical polyadic decomposition[10] as

$$V(q_1,\dots,q_f) = \sum_{r=1}^{R} c_r \prod_{\kappa} \vartheta_{r,\kappa}(q_\kappa), \qquad \text{S1}$$

where $q_\kappa$ are (logical) coordinates, $c_r$ are expansion coefficients and $\vartheta$ are basis functions. The basis functions are not required to be orthogonal, which allows for a very compact representation of the surfaces.

The generation of the decomposition is performed using a Monte-Carlo variant (MCCPD) of the alternating least squares (ALS) algorithm as outlined in Ref. [11].

### A. HBB surface

The PES from Ref. [12] has been fitted with $R = 2048$ terms. All symmetries have been implemented as in Ref. [11]. The PES differs from Ref. [11] by the use of more terms and thus a slightly higher accuracy. TTNS-based reoptimization of the first 239 states on the PES from Ref. [11] leads to differences in the frequencies of max. 3.5 $\mathrm{cm}^{-1}$.

The sampling points for the Monte-Carlo integration within the ALS algorithm were created with a Metropolis algorithm such they resemble a Boltzmann distribution

$$W(q_1,\dots,q_f) = \exp\left(\beta V(q_1,\dots,q_f)\right) \qquad \text{S2}$$

where $\beta = 1/k_\mathrm{B}T$ may be interpreted as an inverse temperature $T$ with $k_\mathrm{B}$ being the Boltzmann constant.

In the present case three different sets of sampling points, each containing $10^6$ points, have been created with a Metropolis algorithm at inverse temperatures of $1/\beta$ =1000 $\mathrm{cm}^{-1}$, $1/\beta$ =2000 $\mathrm{cm}^{-1}$ and $1/\beta$ =4000 $\mathrm{cm}^{-1}$. These sets have been subsequently combined into one single set for creating the fit.

The validation of the fit was performed using independent path integral molecular dynamics (PIMD) configurations generated with the same settings as in Ref. [13]; see the next Section S4 B for details. The mean and root-mean-square (RMS) errors obtained with the validation sets for different temperatures are outlined in Table S4.

All three dipole moment surfaces, $\mu_x$, $\mu_y$, and $\mu_z$, have been fitted with $R = 1024$ terms using the same sampling points as for generating the PES fit. The obtained errors using the same validation sets as for the PES fit are given in Table S5.

### B. BBSM surface

The PES[14] and dipole moments[15] have been fitted using PIMD configurations from Ref. [14] as sampling points. The sets of PIMD configurations have been created at different temperatures from 1.6K to 300K as outlined in Tables S6 and S7.

TABLE S4. Errors of the HBB PES MCCPD (sum-of-products) representation.

| Test temperature $T$ [K] | | Errors [cm$^{-1}$] |
|---|---|---|
| 1.6 | mean | 0.1 |
| | RMS | 9.7 |
| 5 | mean | 0.0 |
| | RMS | 9.9 |
| 10 | mean | 0.0 |
| | RMS | 9.9 |
| 20 | mean | 0.0 |
| | RMS | 9.9 |
| 50 | mean | 0.1 |
| | RMS | 10.3 |
| 100 | mean | 0.2 |
| | RMS | 10.3 |
| 200 | mean | 0.2 |
| | RMS | 10.8 |
| 250 | mean | 0.2 |
| | RMS | 11.1 |
| 300 | mean | 0.1 |
| | RMS | 11.4 |

TABLE S5. Errors of the HBB DMS MCCPD (sum-of-products) representation.

| Test temperature | | Errors [10$^{-4}$ Debye] | | |
|---|---|---|---|---|
| $T$ [K] | | $\mu_x$ | $\mu_y$ | $\mu_z$ |
| 1.6 | mean | 0.0 | 0.2 | 0.0 |
| | RMS | 3.7 | 3.5 | 4.6 |
| 5 | mean | 0.1 | 0.2 | 0.1 |
| | RMS | 3.8 | 3.7 | 4.7 |
| 10 | mean | 0.1 | 0.2 | 0.1 |
| | RMS | 3.8 | 3.5 | 4.7 |
| 20 | mean | 0.1 | 0.2 | 0.0 |
| | RMS | 3.8 | 3.5 | 4.7 |
| 50 | mean | 0.1 | 0.3 | 0.1 |
| | RMS | 3.9 | 3.8 | 5.0 |
| 100 | mean | 0.1 | 0.2 | 0.1 |
| | RMS | 3.9 | 3.8 | 5.0 |
| 200 | mean | 0.1 | 0.2 | 0.1 |
| | RMS | 4.2 | 4.0 | 5.2 |
| 250 | mean | 0.1 | 0.1 | 0.1 |
| | RMS | 4.3 | 4.2 | 5.4 |
| 300 | mean | 0.1 | 0.2 | 0.1 |
| | RMS | 4.4 | 4.3 | 5.5 |

$10^4$ points from each temperature set have been merged into a single set for creating the fits. $3{\cdot}10^5$ different points from each set have been used for validation. The errors obtained with the validation sets are outlined in Tables S6 and S7. All fits (PES and DMS) have been created with $R = 400$ terms. We attribute the slightly worse fitting accuracy of the BBSM DMS to the usage of fewer terms in the MCCPD representation as compared to the HBB DMS. As further validation of the DMSs, we computed the intensities of the eigenfunctions computed on the BBSM PES using both the HBB and BBSM DMSs. We could not find any significant difference, indicating that, for the DMS, not only the MCCPD fits but also the two DMSs are of similar, high quality.

TABLE S6. Errors of the BBSM PES MCCPD (sum-of-products) representation.

| Test temperature $T$ [K] | | Errors [cm$^{-1}$] |
|---|---|---|
| 1.6 | mean | 0.0 |
| | RMS | 6.0 |
| 5 | mean | 0.0 |
| | RMS | 5.9 |
| 10 | mean | 0.0 |
| | RMS | 5.9 |
| 20 | mean | 0.0 |
| | RMS | 6.0 |
| 50 | mean | 0.0 |
| | RMS | 6.8 |
| 100 | mean | 0.0 |
| | RMS | 7.0 |
| 200 | mean | 0.0 |
| | RMS | 8.0 |
| 250 | mean | 0.0 |
| | RMS | 9.4 |
| 300 | mean | 0.0 |
| | RMS | 10.9 |

TABLE S7. Errors of the BBSM DMS MCCPD (sum-of-products) representation.

| Test temperature | | Errors [10$^{-4}$ Debye] | | |
|---|---|---|---|---|
| $T$ [K] | | $\mu_x$ | $\mu_y$ | $\mu_z$ |
| 1.6 | mean | 0.0 | 0.0 | 0.0 |
| | RMS | 13.3 | 11.9 | 42.6 |
| 5 | mean | 0.0 | 0.0 | -0.1 |
| | RMS | 13.3 | 11.9 | 42.7 |
| 10 | mean | 0.0 | 0.1 | -0.2 |
| | RMS | 13.3 | 11.8 | 42.6 |
| 20 | mean | 0.0 | 0.0 | -0.1 |
| | RMS | 13.2 | 11.9 | 42.5 |
| 50 | mean | 0.0 | -0.1 | -0.3 |
| | RMS | 13.8 | 12.6 | 43.9 |
| 100 | mean | 0.0 | 0.0 | -0.2 |
| | RMS | 14.5 | 13.0 | 45.4 |
| 200 | mean | 0.1 | 0.0 | -0.2 |
| | RMS | 16.4 | 14.3 | 48.8 |
| 250 | mean | 0.1 | 0.0 | 0.0 |
| | RMS | 18.1 | 15.5 | 51.3 |
| 300 | mean | 0.2 | 0.0 | -0.1 |
| | RMS | 18.9 | 16.2 | 53.8 |

## S5. COMPARISON WITH AB INITIO DATA

In order to provide a fair reference for the comparison of the two PESs and the MCCPD fits of these PESs, for a sample of configurations, we compare the energies of the PESs with electronic structure energies. The electronic structure ener-

gies were performed using basis set extrapolated coupled cluster singles and doubles with perturbative triples, CCSD(T), calculations. For that purpose, canonical CCSD(T)/aug-cc-pVTZ and CCSD(T)/aug-cc-pVQZ correlation energies were extrapolated using the formula $E_n = E_{\mathrm{CBS}} + a/n^3$,[16,17] where $n$ is the cardinal number and $a$ a parameter; denoted as CCSD(T)/CBS[34]. Hartree–Fock energies were not extrapolated but taken directly from the larger basis set.

The samples were obtained by randomly selecting configurations from diffusion Monte Carlo runs.[18] For the two PESs we selected each 1000 configurations from runs each with 4000 Monte Carlo walkers and $10^4$ time steps (plus $10^3$ equilibrium steps) of size 10 a.u. Since the MCCPD fit is only valid on the grid, we mapped these configurations onto the grid and removed those that are outside the grid. We obtained 889 (957) configurations on the HBB (BBSM) PES, for which explicit CCSD(T)/CBS[34] calculations were performed.

The combined configurations are used for estimating the accuracy of the PESs in Fig. S3 A-C. Both PESs have very good accuracy but the newer BBSM PES is twice as accurate as the HBB PES. For the HBB PES for the configurations we obtain a mean absolute error (MAE) of 203 $\mathrm{cm}^{-1}$, whereas for the BBSM PES we obtain a better accuracy with an MAE of 75 $\mathrm{cm}^{-1}$. We note in passing that the reference method used for the BBSM PES (CCSD(T$*$)-F12a/AVTZ) is expected to be closer to the absolute basis set limit than the CBS[34] results[19] suggesting in practice an even better performance of that PES. We obtain similar results when analyzing the 1000 configurations from each PES separately.

The MCCPD energies are then compared with the energies from the PES. Note that this analysis is independent from Sections S4 A and S4 B as different samples and error measures are used, thus providing an additional stringent validation test. The accuracy of the MCCPD refits using these 1846 configurations is shown in Fig. S3 D-F. For the HBB MCCPD we obtain an MAE of 16 $\mathrm{cm}^{-1}$, whereas for the BBSM MCCPD we obtain an MAE of 13 $\mathrm{cm}^{-1}$. In addition to this analysis, we compared the MCCPD directly with the CCSD(T)/CBS[34] energies (not shown in Fig. S3). Then, for the HBB MCCPD we obtain an MAE of 203 $\mathrm{cm}^{-1}$, whereas for the BBSM MCCPD we obtain an MAE of 76 $\mathrm{cm}^{-1}$. Both of these MAEs are very similar to the benchmark of the original PESs, indicating error cancellation between basis set incompleteness, as well as PES and MCCPD fitting accuracy. The MCCPD fits are excellent and, given the finite accuracy of the original PES fits, do not decrease the accuracy, compared to the electronic structure energies.

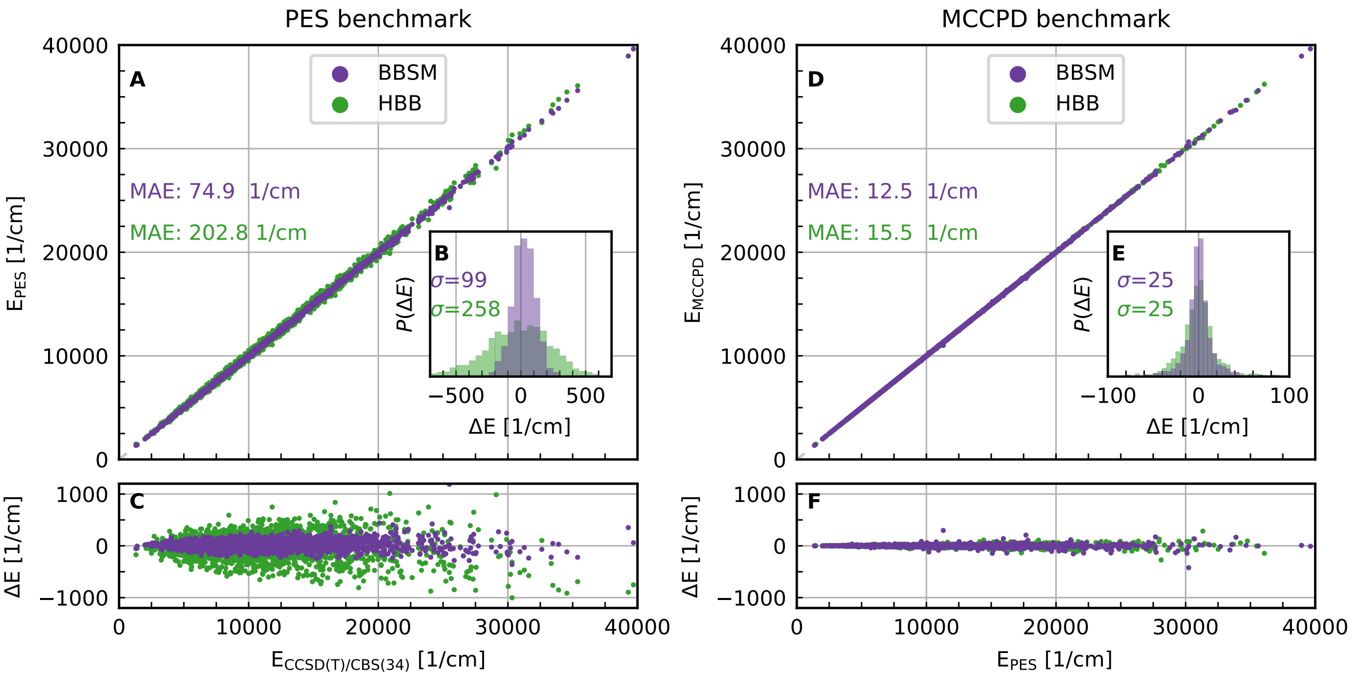


FIG. S3. Benchmark of the PES fits (panels A-C) and the MCCPD refits (panels D-F). The PES energies are compared with CCSD(T)/CBS[34] energies, whereas the MCCPD energies are compared with the PES energies for around 2000 configurations. Panels A and D: Correlation of the fitted energies, where mean absolute errors (MAE) for both surfaces are stated in the respective color. Panels B and E: Histogram of the energy differences including the corresponding standard deviations ($\sigma$) in the respective color. Panels C and F: Energy differences between reference and prediction over the whole range of reference energies.

[1]O. Vendrell, F. Gatti, and H.-D. Meyer, "Full dimensional (15-dimensional) quantum-dynamical simulation of the protonated water dimer. II. Infrared spectrum and vibrational dynamics," J. Chem. Phys. **127**, 184303 (2007).

[2]O. Vendrell, M. Brill, F. Gatti, D. Lauvergnat, and H.-D. Meyer, "Full dimensional (15-dimensional) quantum-dynamical simulation of the protonated water-dimer III: Mixed Jacobi-valence parametrization and benchmark results for the zero point energy, vibrationally excited states, and infrared spectrum," J. Chem. Phys. **130**, 234305 (2009).

[3]O. Vendrell, F. Gatti, and H.-D. Meyer, "Full dimensional (15 dimensional) quantum-dynamical simulation of the protonated water-dimer IV: Isotope effects in the infrared spectra of $D(D_2O)^{2+}$, $H(D_2O)^{2+}$, and $D(H_2O)^{2+}$ isotopologues," J. Chem. Phys. **131**, 034308 (2009).

[4]H. R. Larsson, "Computing vibrational eigenstates with tree tensor network states (TTNS)," J. Chem. Phys. **151**, 204102 (2019).

[5]H. R. Larsson, H. Zhai, K. Gunst, and G. K.-L. Chan, "Matrix Product States with Large Sites," J. Chem. Theory Comput. **18**, 749–762 (2022).

[6]J. Haegeman, C. Lubich, I. Oseledets, B. Vandereycken, and F. Verstraete, "Unifying time evolution and optimization with matrix product states," Phys. Rev. B **94**, 165116 (2016).

[7]F. A. Y. N. Schröder, D. H. P. Turban, A. J. Musser, N. D. M. Hine, and A. W. Chin, "Tensor network simulation of multi-environmental open quantum dynamics via machine learning and entanglement renormalisation," Nat. Commun. **10**, 1062 (2019).

[8]U. Schollwöck, "The density-matrix renormalization group in the age of matrix product states," Ann. Phys. **326**, 96–192 (2011).

[9]O. Vendrell, F. Gatti, and H.-D. Meyer, "Dynamics and Infrared Spectroscopy of the Protonated Water Dimer," Angew. Chem. Int. Ed. **46**, 6918–6921 (2007).

[10]F. L. Hitchcock, "The expression of a tensor or a polyadic as a sum of products," J. Math. Phys. **6**, 164–189 (1927).

[11]M. Schröder, "Transforming high-dimensional potential energy surfaces into a canonical polyadic decomposition using Monte Carlo methods," J. Chem. Phys. **152**, 024108 (2020).

[12]X. Huang, B. J. Braams, and J. M. Bowman, "*Ab Initio* potential energy and dipole moment surfaces for $H_5O_2^+$," J. Chem. Phys. **122**, 044308 (2005).

[13]C. Schran and D. Marx, "Quantum nature of the hydrogen bond from ambient conditions down to ultra-low temperatures," Phys. Chem. Chem. Phys. **21**, 24967–24975 (2019).

[14]C. Schran, J. Behler, and D. Marx, "Automated fitting of neural network potentials at coupled cluster accuracy: Protonated water clusters as testing ground," J. Chem. Theory Comput. **16**, 88–99 (2020).

[15]R. Beckmann, F. Brieuc, C. Schran, and D. Marx, "Infrared spectra at coupled cluster accuracy from neural network representations," J. Chem. Theory Comput. , in press (2022).

[16]T. Helgaker, W. Klopper, H. Koch, and J. Noga, "Basis-set convergence of correlated calculations on water," J. Chem. Phys. **106**, 9639–9646 (1997).

[17]K. L. Bak, P. Jørgensen, J. Olsen, T. Helgaker, and W. Klopper, "Accuracy of atomization energies and reaction enthalpies in standard and extrapolated electronic wave function/basis set calculations," J. Chem. Phys. **112**, 9229–9242 (2000).

[18]J. B. Anderson, "A random-walk simulation of the Schrödinger equation: $H_3{}^+$," J. Chem. Phys. **63**, 1499–1503 (1975).

[19]T. B. Adler, G. Knizia, and H.-J. Werner, "A simple and efficient CCSD(T)-F12 approximation," J. Chem. Phys. **127**, 221106 (2007).
